# Supplementary material for: A modular architecture for transparent computation in Recurrent Neural Networks
Source: arXiv:1609.01926 ancillary file (2016-09-07)
Supplement: Supplementary file 1 [file supplementary.pdf]

# Supplementary Materials for "A modular architecture for transparent computation in Recurrent Neural Networks"

In what follows, we will use a prefix "M." when referring to material in the main paper.

## 1 Example: Odd vs Even Turing Machine

To review the different stages of our methodology concerning Turing Machines (and thus to show the universality of our architecture) we present a simple example. Consider a TM that accepts unary strings containing an even number of `1`'s, and rejects those containing an odd number of `1`'s. The set of states of the machine is specified by $Q = \{q_{\text{even}}, q_{\text{odd}}, q_{\text{acc}}, q_{\text{rej}}\}$, where $q_{\text{even}}$ is the initial state, $q_{\text{acc}}$ is the accept state and $q_{\text{rej}}$ is the reject state. The set of tape symbols is $\mathbf{N} = \{\sqcup, \mathtt{1}\}$, and the $\delta$ transition function is presented in Table 1. A VS simulating this machine is constructed as shown in Section M.2.1.1, and Gödelized as shown in Section M.2.2.1. Specifically, the Gödelization for the left part of the dotted sequence encoding TM configurations can be defined as in Equation M.19 (as the configurations always contain a state as the first symbol, and tape symbols thereafter), whereas the right part can be Gödelized as in Equation M.18, leading to the following encodings:

$$\psi_x(s) := \gamma_q(d_1)n_q^{-1} + \sum_{k=1}^{\infty} \gamma_s(d_{k+1})n_s^{-k}n_q^{-1}, \qquad \psi_y(s) := \sum_{k=1}^{\infty} \gamma_s(d_k)n_s^{-k},$$

where $\gamma_q$ and $\gamma_s$ respectively enumerate states and tape symbols, $n_q = |Q|$ and $n_s = |\mathbf{N}|$ are the number of states and tape symbols, and $d_i$ is the $i$-th

| Symbols | States | |
|---|---|---|
| | $q_{\text{even}}$ | $q_{\text{odd}}$ |
| `1` | $(q_{odd}, \mathtt{1}, \mathcal{R})$ | $(q_{even}, \mathtt{1}, \mathcal{R})$ |
| $\sqcup$ | $(q_{acc}, \sqcup, \mathcal{L})$ | $(q_{rej}, \sqcup, \mathcal{L})$ |

Table 1: **State transition table for the odd vs even string Turing machine.** The table represents the action of the $\delta$ transition function (i.e. Equation M.13). For example, if the machine is in state $q_{even}$ and receives as input a `1`, then the Turing machine writes a `1` on the tape, then it transitions to state $q_{odd}$ and finally moves the machines' control head to the right ($\mathcal{R}$).

symbol in the subsequence to Gödelize. Specifically, the $\gamma_q, \gamma_s$ enumerations are defined as follows:

$$\gamma_q := \{(\sqcup, 0), (\mathtt{1}, 1)\}$$
$$\gamma_s := \{(q_{\text{acc}}, 0), (q_{\text{rej}}, 1), (q_{\text{even}}, 2), (q_{\text{odd}}, 3)\}$$

where each enumerating function is represented as a set of pairs $(d, k)$, where $d$ is a symbol and $k \in \mathbb{N}$ its enumeration. Gödelizing the VS defines a NDA on the unit square, with affine-linear transformations parameters derived as in Section M.2.2.2. The NDA can then be mapped to a R-ANN following the methods presented in Section M.2.3, resulting in a network of 45 neural units (see Equation M.33). The simulation of the R-ANN is depicted in Figure 1, where it is possible to observe the activation values of the MCL neurons at each time step for respectively an input string of `1111` and one of `111`. By decoding these activation values the tape dynamics of the simulated TM can be retrieved as shown in Figure 2. Note in particular how the final states on the unit square lay respectively on a $q_{\text{accept}}$ and $q_{\text{rej}}$ cell. These are the halting states of the TM, mapping in this example to a fixed point halting condition. Note that the methodology employed in this simple example can be applied to the mapping of any arbitrary Turing machine to the proposed R-ANN architecture. The process simply becomes a question of substituting the details of the TM presented in this example (i.e. the set of states, the set of tape symbols and the transition function) to that of the desired machine, obtaining a R-ANN that simulates it in real-time.

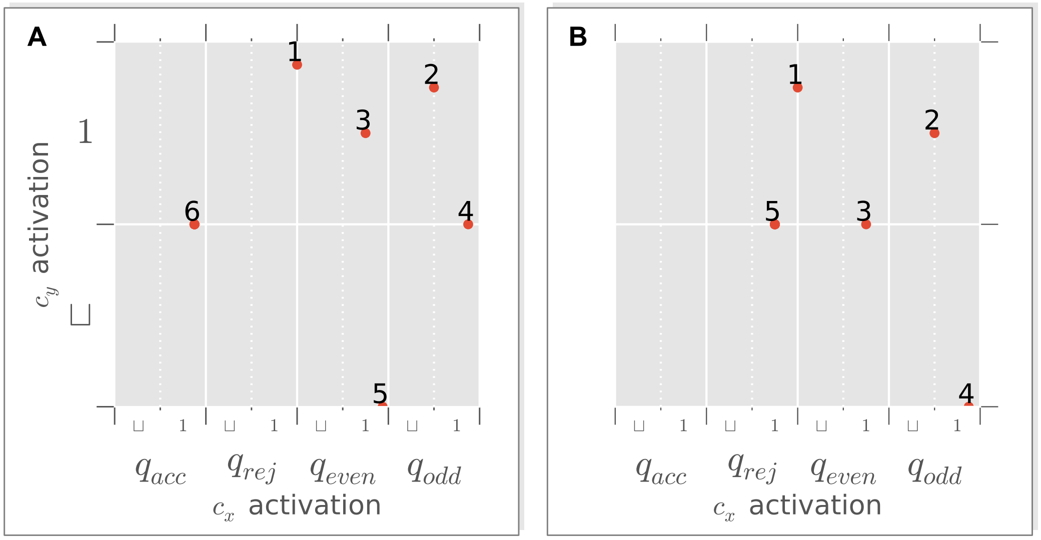


Figure 1: **Dynamics on the unit square of neural unit activations in the machine configuration layer.** (A) Dynamics for an input encoding a string containing an even number of `1`'s. Each point corresponds to a computation step in the recurrent artificial neural network, and is numbered accordingly. The $x$ and $y$ values for each point correspond respectively to the activation of the $c_x$ and $c_y$ machine configuration layer units. The unit square is partitioned as in the simulated nonlinear dynamical automaton to highlight the relation between the unit activations and the underlying symbolic dynamics. It is possible to recognize the alternation between the $q_{\text{even}}$ and $q_{\text{odd}}$ states and the final state reached at the end of the computation. The computation halts on an accept state, as the encoded input string is even. (B) The input encodes an odd string, consequently the computation halts on a reject state.

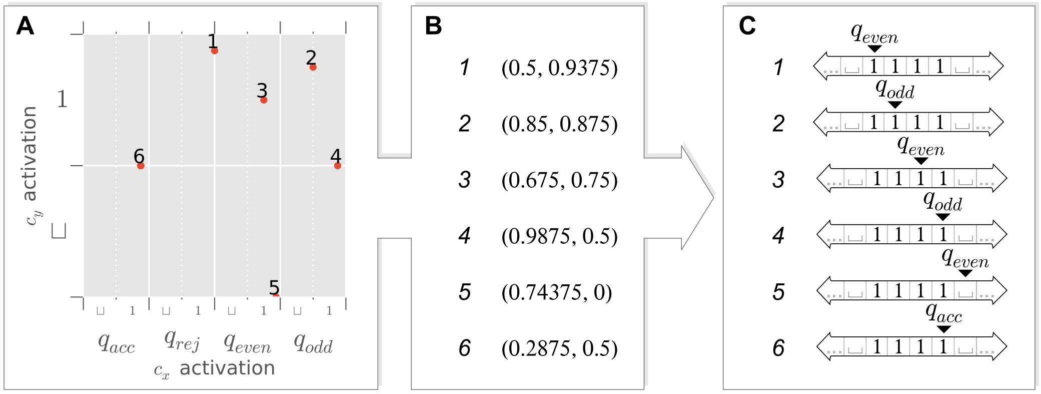


Figure 2: **Decoding of Turing machine configurations from machine configuration layer activations.** The simulated Turing machine dynamics (C) can be decoded from the activations (B) of the $c_x$ and $c_y$ units in the machine configuration layer at each time step. The figure also highlights the equivalence between the representation used in Figure 1, visualizing the computation as point dynamics on the unit square (A), and as a nsequence of machine configuration layer units activations (B).

# References


Moore, C. (1990). Unpredictability and undecidability in dynamical systems. *Physical Review Letters*, 64(20):2354 – 2357.

Moore, C. (1991). Generalized shifts: unpredictability and undecidability in dynamical systems. *Nonlinearity*, 4:199 – 230.

Sipser, M. (2006). *Introduction to the Theory of Computation*. Thomson Course Technology Boston.

Turing, A. M. (1937). On computable numbers, with an application to the *Entscheidungsproblem*. *Proceedings of the London Mathematical Society*, 42.
